# Supplementary material for: ReMoE: An Interpretable Mixture-of-Experts Framework for Human Mobility Recovery Forecasting Across Disasters
Source: arXiv:2611.22133 source file (2026-11-17)
Supplement: Supplementary file 1 [file supplement_table.tex]

% \begin{table*}[p]
% \centering
% \small
% \setlength{\tabcolsep}{2.5pt}
% \renewcommand{\arraystretch}{1.08}

% \caption{Event-level ReMoE performance under LOEO and LOHTO evaluation.}
% \label{tab:app-event-performance}

% \newcommand{\scorepm}[2]{#1\,{\scriptsize\(\pm\)}\,#2}

% \begin{tabular*}{\textwidth}{
% @{}
% >{\centering\arraybackslash}p{0.95cm}@{\hspace{3pt}}
% >{\raggedright\arraybackslash}p{4.10cm}@{\hspace{4pt}}
% >{\centering\arraybackslash}p{0.95cm}
% @{\extracolsep{\fill}}
% ccccc
% @{}
% }
% \toprule
% \textbf{Setting}
% & \textbf{Held-out event}
% & \(\mathbf{N}_e\)
% & \textbf{RMSE\(\downarrow\)}
% & \textbf{MAE\(\downarrow\)}
% & \textbf{\(R^2\uparrow\)}
% & \textbf{CDE\(\downarrow\)}
% & \textbf{RTE\(\downarrow\)} \\
% \midrule

% \multirow{22}{*}{\textbf{LOEO}}
% & \multicolumn{7}{@{}l}{\textbf{Hurricanes}} \\[-1pt]
% & Dorian (2019) & 24  & 0.082 & 0.066 & 0.612 & 0.348 & 1.145 \\
% & Laura (2020) & 464 & 0.071 & 0.055 & 0.725 & 0.270 & 0.884 \\
% & Ida (2021) & 403 & 0.063 & 0.048 & 0.748 & 0.241 & 0.812 \\
% & Nicholas (2021) & 127 & 0.057 & 0.045 & 0.775 & 0.224 & 0.768 \\
% & Ian (2022) & 341 & 0.064 & 0.050 & 0.738 & 0.251 & 0.842 \\
% & Francine (2024) & 398 & 0.069 & 0.053 & 0.720 & 0.269 & 0.896 \\
% & Helene (2024) & 211 & 0.075 & 0.059 & 0.662 & 0.307 & 1.006 \\
% & Milton (2024) & 491 & 0.061 & 0.047 & 0.690 & 0.270 & 0.941 \\

% \cmidrule(lr){2-8}
% & \multicolumn{7}{@{}l}{\textbf{Winter storms}} \\[-1pt]
% & Uri (2021) & 786
% & \scorepm{0.072}{0.003} & \scorepm{0.056}{0.002}
% & \scorepm{0.696}{0.016} & \scorepm{0.272}{0.012}
% & \scorepm{0.955}{0.037} \\
% & Buffalo lake-effect snowstorm (2022) & 185
% & \scorepm{0.074}{0.004} & \scorepm{0.058}{0.003}
% & \scorepm{0.681}{0.021} & \scorepm{0.281}{0.014}
% & \scorepm{0.989}{0.044} \\
% & January winter storm (2024) & 374
% & \scorepm{0.076}{0.004} & \scorepm{0.060}{0.003}
% & \scorepm{0.651}{0.019} & \scorepm{0.296}{0.012}
% & \scorepm{1.018}{0.047} \\
% & January winter storm (2025) & 543
% & \scorepm{0.079}{0.005} & \scorepm{0.063}{0.004}
% & \scorepm{0.612}{0.026} & \scorepm{0.301}{0.018}
% & \scorepm{1.058}{0.054} \\

% \cmidrule(lr){2-8}
% & \multicolumn{7}{@{}l}{\textbf{Floods}} \\[-1pt]
% & KY--MO riverine flood (2022) & 391
% & \scorepm{0.075}{0.005} & \scorepm{0.061}{0.004}
% & \scorepm{0.650}{0.024} & \scorepm{0.301}{0.015}
% & \scorepm{0.996}{0.052} \\
% & Vermont--New York flood (2023) & 108
% & \scorepm{0.081}{0.006} & \scorepm{0.065}{0.005}
% & \scorepm{0.610}{0.031} & \scorepm{0.319}{0.020}
% & \scorepm{1.104}{0.071} \\

% \cmidrule(lr){2-8}
% & \multicolumn{7}{@{}l}{\textbf{Wildfires}} \\[-1pt]
% & Saddleridge (2019) & 27
% & \scorepm{0.069}{0.005} & \scorepm{0.056}{0.004}
% & \scorepm{0.704}{0.027} & \scorepm{0.257}{0.018}
% & \scorepm{0.980}{0.059} \\
% & August Complex (2020) & 88
% & \scorepm{0.071}{0.004} & \scorepm{0.058}{0.003}
% & \scorepm{0.685}{0.025} & \scorepm{0.271}{0.017}
% & \scorepm{1.021}{0.051} \\
% & Lahaina (2023) & 45
% & \scorepm{0.086}{0.007} & \scorepm{0.073}{0.006}
% & \scorepm{0.565}{0.041} & \scorepm{0.351}{0.027}
% & \scorepm{1.180}{0.086} \\
% & Palisades--Eaton (2025) & 25
% & \scorepm{0.082}{0.006} & \scorepm{0.071}{0.005}
% & \scorepm{0.626}{0.035} & \scorepm{0.319}{0.024}
% & \scorepm{1.099}{0.074} \\

% \midrule

% \multirow{26}{*}{\textbf{LOHTO}}
% & \multicolumn{7}{@{}l}{\textbf{Hurricanes}} \\[-1pt]
% & Dorian (2019) & 24  & 0.091 & 0.076 & 0.571 & 0.371 & 1.181 \\
% & Laura (2020) & 464 & 0.073 & 0.061 & 0.704 & 0.269 & 0.903 \\
% & Ida (2021) & 403 & 0.069 & 0.058 & 0.727 & 0.254 & 0.861 \\
% & Nicholas (2021) & 127 & 0.066 & 0.055 & 0.754 & 0.238 & 0.817 \\
% & Ian (2022) & 341 & 0.074 & 0.062 & 0.706 & 0.276 & 0.934 \\
% & Francine (2024) & 398 & 0.078 & 0.065 & 0.688 & 0.298 & 0.976 \\
% & Helene (2024) & 211 & 0.084 & 0.070 & 0.638 & 0.332 & 1.117 \\
% & Milton (2024) & 491 & 0.081 & 0.065 & 0.684 & 0.298 & 1.067 \\

% \cmidrule(lr){2-8}
% & \multicolumn{7}{@{}l}{\textbf{Winter storms}} \\[-1pt]
% & Uri (2021) & 786 & 0.081 & 0.067 & 0.657 & 0.323 & 1.028 \\
% & Buffalo lake-effect snowstorm (2022) & 185 & 0.076 & 0.062 & 0.692 & 0.298 & 0.972 \\
% & January winter storm (2024) & 374 & 0.082 & 0.069 & 0.648 & 0.331 & 1.061 \\
% & January winter storm (2025) & 543 & 0.089 & 0.074 & 0.567 & 0.364 & 1.183 \\

% \cmidrule(lr){2-8}
% & \multicolumn{7}{@{}l}{\textbf{Floods}} \\[-1pt]
% & KY--MO riverine flood (2022) & 391 & 0.083 & 0.069 & 0.624 & 0.336 & 1.083 \\
% & Vermont--New York flood (2023) & 108 & 0.087 & 0.073 & 0.590 & 0.352 & 1.153 \\

% \cmidrule(lr){2-8}
% & \multicolumn{7}{@{}l}{\textbf{Wildfires}} \\[-1pt]
% & Saddleridge (2019) & 27 & 0.081 & 0.067 & 0.618 & 0.346 & 1.087 \\
% & August Complex (2020) & 88 & 0.087 & 0.072 & 0.573 & 0.367 & 1.136 \\
% & Lahaina (2023) & 45 & 0.097 & 0.081 & 0.482 & 0.429 & 1.319 \\
% & Palisades--Eaton (2025) & 25 & 0.087 & 0.072 & 0.599 & 0.358 & 1.126 \\

% \bottomrule
% \end{tabular*}

% \vspace{2pt}
% \begin{minipage}{\textwidth}
% \footnotesize
% \textit{Note.} \(N_e=|\mathcal R_e|\) is the number of tract--event samples
% for event \(e\). Under LOEO, repeated held-out events are summarized across rotations, with standard deviations reflecting changes in training-event composition.
% \end{minipage}
% \end{table*}
